# Supplementary material for: Nanometer-scale Tomographic Reconstruction of 3D Electrostatic Potentials in GaAs/AlGaAs Core-Shell Nanowires
Source: arXiv:1407.1781 source file (2014-07-07)
Supplement: Supplementary file 1 [file Supplement.pdf]

# Supplementary Information

## Nanometer-scale Tomographic Reconstruction of 3D Electrostatic Potentials in GaAs/AlGaAs Core-Shell Nanowires


A. Lubk, D. Wolf, S. Sturm, and H. Lichte

*Triebenberg Laboratory, Institute of Structure Physics, Technische Universität Dresden, 01062 Dresden, Germany*

P. Prete

*IMM-CNR, Lecce Research Unit, S.P. 6 Lecce-Monteroni, I-73100, Lecce, Italy*

N. Lovergine

*Dipartimento di Ingegneria dell'Innovazione, Università del Salento, S.P. 6 Lecce-Monteroni, I-73100 Lecce, Italy*

T. Niermann

*Institut für Optik und Atomare Physik, Technische Universität Berlin, Straße des 17. Juni 135, 10623 Berlin, Germany*

## I. RADON TRANSFORMATION AND SAMPLING

In the main text we used a polar sampling of reconstruction space for the algebraic formulation of the Radon Transformation. That had several advantages like minimizing the number of sampling points and incorporating radial symmetries. In the following we will supplement how the polar sampling naturally derives from a particular formulation of the Radon Transformation separated into angular and radial coordinates. The separation facilitates a separated application of the (generalized) Shannon-Nyquist sampling theorem eventually leading to the polar grid as preferential sampling. In the course of these considerations it will also become clear why the axis with the smallest azimuthal band should be chosen as origin of the polar grid.

We will denote the Radon transform of a function $f$ by $\hat{f}$ and employ the coordinate system given in the main text ($p\epsilon\,[-\infty,\infty]$,$\theta\epsilon\,[0,\pi]$, see Fig. 3 of the main text). With $\Omega$ denoting the reconstruction domain the line integrals (1) can then be reformulated in the following way

$$\begin{aligned} \hat{f}\left(p,\theta\right) &= \iint_{\Omega} f\left(y,z\right)\delta\left(p-y\cos\theta-z\sin\theta\right)\mathrm{d}y\mathrm{d}z \\ &= \int_0^{\infty}\int_0^{2\pi} f\left(r,\varphi\right)\delta\left(p-r\cos\left(\theta-\varphi\right)\right)r\mathrm{d}r\mathrm{d}\varphi\,. \end{aligned} \tag{1}$$

Note that the polar formulation in the second line contains a convolution in the angular coordinate. The projection operation along continuous tilt angles is invertible under relatively weak conditions, including the experimentally relevant one that the function $f\left(y,z\right)$ is continuous and vanishes outside the bounded reconstruction domain $\Omega$ (e.g. [3]). The pair of forward and backward transformation is called Radon and inverse Radon transformation ([4]). Several explicit analytic expressions have been derived for these pairs [3] and we will proceed with deriving the, in a certain sense, most symmetric one. The starting point is the second line of (1), where we insert the Fourier expansion of

$$f\left(r,\varphi\right)=\sum_{n=-\infty}^{\infty} f_n\left(r\right)e^{in\varphi} \tag{2}$$

with expansion coefficients

$$f_n\left(r\right)=\frac{1}{2\pi}\int_0^{2\pi} f\left(r,\varphi\right)e^{-in\varphi}d\varphi \tag{3}$$

into circular harmonics

$$\begin{aligned}\hat{f}(p,\theta) &= \int_0^\infty \int_0^{2\pi} \sum_{n=-\infty}^{\infty} f_n(r)\, e^{in\varphi} \delta\left(p - r\cos\left(\theta-\varphi\right)\right) r\mathrm{d}r\mathrm{d}\varphi \\ &= \sum_{n=-\infty}^{\infty} \int_0^\infty \int_0^{2\pi} f_n(r)\, e^{in\varphi} \delta\left(p - r\cos\left(\theta-\varphi\right)\right) r\mathrm{d}r\mathrm{d}\varphi\end{aligned} \tag{4}$$

and exchange summation and integration on the second line. In the next step we Fourier transform both sides along the $p$-coordinate, exchange the integration order and carry out the $p$-integration

$$\begin{aligned}\hat{\mathfrak{f}}(q,\theta) &= \int \hat{f}(p,\theta)\, e^{-iqp}\mathrm{d}p \\ &= \sum_{n=-\infty}^{\infty} \int_0^\infty \int_0^{2\pi} \int f_n(r)\, e^{in\varphi} \delta\left(p - r\cos\left(\theta-\varphi\right)\right) e^{-iqp} r\mathrm{d}r\mathrm{d}\varphi\mathrm{d}p \\ &= \sum_{n=-\infty}^{\infty} \int_0^\infty \int_0^{2\pi} f_n(r)\, e^{in\varphi} e^{-iqr\cos(\theta-\varphi)} r\mathrm{d}r\mathrm{d}\varphi\,.\end{aligned} \tag{5}$$

In a final step we insert the following identity for the Bessel function

$$J_n(qr) = \frac{1}{2\pi i^n} \int_0^{2\pi} e^{in\varphi} e^{iqr\cos\varphi}\mathrm{d}\varphi\,. \tag{6}$$

We furthermore slightly change the definition of $q$ and $\theta$ to true polar coordinates

$$q', \theta' = \begin{cases} q, \theta & q \geq 0 \\ -q, \theta + \pi & q < 0 \end{cases} \tag{7}$$

obtaining

$$\hat{\mathfrak{f}}(q', \theta') = \sum_{n=-\infty}^{\infty} e^{in\theta} \mathfrak{f}_n(q') \tag{8}$$

with

$$\mathfrak{f}_n(q') = 2\pi i^n \int_0^\infty f_n(r)\, J_n(q'r)\, r\mathrm{d}r\,. \tag{9}$$

Thus the harmonic expansion coefficients of the original function and the Fourier transform of the projected data are connected by a Hankel transformation. The latter is an invertible transformation pair according to

$$f_n(r) = 2\pi i^{-n} \int_0^\infty \mathfrak{f}_n(q')\, J_n(q'r)\, q'\mathrm{d}q'\,. \tag{10}$$

Consequently, expressions (2),(8),(9) and (10) yield a symmetric version of the Radon transformation (e.g. [1]) with the nice property that azimuthal and radial coordinates are separated.

This last property facilitates a discussion of sampling in azimuthal and radial coordinates separately. The radial case concerns the requirements for the detector sampling in order to obtain $f_n(r)$. That problem is involved and requires generalized sampling theorems [2]. Here, we will assume that radial sampling is sufficient to completely determining $\mathfrak{f}_n(q')$ for evaluating the inverse Hankel transformation (10). For that it is sufficient to demand the function $f$ to be band-limited and sampled accordingly. To discuss the azimuthal sampling we restrict ourselves to the experimental case of equally spaced azimuthal sampling points (i.e. tilt angles). According to the Shannon-Nyquist sampling theorem the tilt increment between tilt angles must then be $\pi/n_{\max}$ or smaller in order to completely represent an azimuthal band-limited signal with maximal frequency $n_{max}/2\pi$. The symmetric Hankel transformation pair now imposes the same condition to the projected data. For the example of a radially symmetric function used in the main text one therefore not only requires only one projection for a complete reconstruction but also only one position space harmonic expansion coefficient. To exploit this reduced harmonic basis the Radon transformation has to be discretized on a polar grid, i.e. in angular and radial coordinates, and not on a Cartesian grid.

So far we used polar coordinates with a deliberately chosen origin. Indeed there is no distinguished origin which corresponds to a free choice of the rotation axis in the reconstruction. However, for different origins the harmonic expansion changes, for instance the radial symmetry of our previous example is only valid around the symmetry point and an infinite harmonic series occurs around other points. So how many tilt angles do we need? The answer depends on which axis we chose for reconstruction: If we are able to pick the symmetry axis (or axis with smallest azimuthal bandwidth in the general case) a small number of tilt angles is sufficient for a complete reconstruction. This is the reason why we aligned the experimental tilt series slice-wise around the center of mass approximately coinciding with the symmetry axis of the NW. Reconstruction on Cartesian grids are shift invariant hence do not distinguish a certain rotation axis. That has the advantage of not requiring to find the axis of smallest azimuthal bandwidth and the disadvantage of eventually reconstructing a significantly larger amount of pixels than actually required (and meaningful).

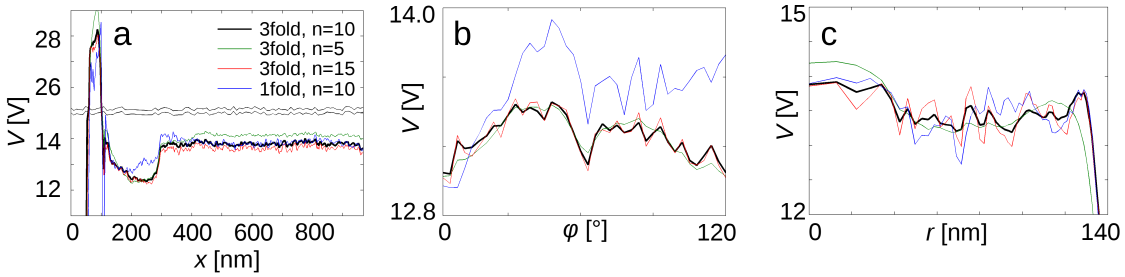


Figure 1: Comparison of different regularization parameter values. Potential linescans corresponding to Fig. 4 in the main text along $x$ (a), azimuth $\varphi$ (b) and $r$ (c).

We finally note that the discrete Radon matrix reflects the analytic structure of the harmonic expansion and the Hankel transformation between the expansion coefficients. For instance the azimuthal convolution in the second line of (1), leads to a Toeplitz structure in the Radon matrix, the diagonalization of which corresponding to the analytical harmonic series expansion. The latter can be accomplished by Fast Fourier techniques, which leads to very fast algorithms comparable to Filtered Techniques (see [3]). In our case we did not diagonalize the azimuthal convolution in order to incorporate symmetry and spatial constrains, applying in position space, in our formalism.

## II. REGULARIZATION AND RECONSTRUCTION

It was stated in the main text that the there is no distinguished regularization parameter value because we do not know the error between the reconstruction and original object. We therefore supplement reconstructions from different regularization parameters. Note that such a comparison is often absent in current literature on tomographic TEM methods affecting the quantitative analysis. Two regularizations have been applied (simultaneously) in the main text: A quasi-Tikhonov regularization parametrized by the number of iterations of the used LSQR algorithm and the requirement of a three-fold symmetry axis.

Fig. 1 shows line scans corresponding to Fig. 4 in the main text obtained from reconstructions with 5, 10 (used in main text) and 15 LSQR iteration cycles as well as from a reconstruction with no symmetry constraint. One readily observes an improvement of spatial resolution at the cost of signal resolution (noise) with growing iteration number.

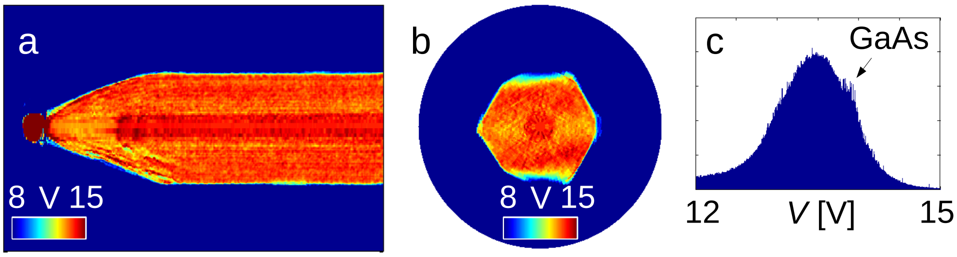


Figure 2: Reconstructed potential without symmetry constraint. The cross-sections in the $xz$-plane (a) and $yz$-plane (b) correspond to the ones shown in Fig. 4 of the main text. The missing wedge shows up as horizontal stripes in b. The histogram of the potential values is shown in c.

For instance the potential drop due to Al enrichment at the nanofacets becomes slightly deeper at 15 LSQR iterations (see Fig. 1) with the value itself being more uncertain due to the increased noise. In detail, the results obtained from 5 iterations revealed a resolution around 8 nm determined from the FWHM of the potential gradient at the NW edge, which subsequently raised to 6 nm at 10 and 15 iterations. At the same time noise started to significantly increase around 15 iterations (see e.g. Fig. 1c), which is why 10 iterations have been judged a good compromise.

The impact of the symmetry constraint is more difficult to assess since the regularization error is introduced by unknown symmetry violations present in the object. We therefore performed a reconstruction without symmetry constraint and 10 LSQR iterations (see Fig. 2 for cross-section corresponding to Fig. 4 in the main text). We obtain large missing wedge artifacts most prominently visible as horizontal lines within the NW in Fig. 2b. Note that these artifacts were present even though the vacuum was blocked from reconstruction by the segmentation of the Radon matrix illustrated in Fig. 3b of the main text. These missing wedge artifacts significantly reduce the signal resolution (see Fig. 2c) and obscure fine potential details such as the Al segregation lines or the precision of the mean inner potential values (see Fig. 1 and 2c in particular). Note, however, that the Al segregation is faintly present in Fig. 1b underlining that they cannot be considered an artifact of the

symmetry constrained reconstruction.


[1] Cormack, A. M., 1963. Representation of a function by its line integrals. with some radiological applications. Journal of Applied Physics 34, 2722–2727.

[2] Jerri, A., 1977. The Shannon sampling theorem - Its various extensions and applications: A tutorial review. Proceedings of the IEEE 65 (11), 1565–1596.

[3] Natterer, F., 2001. The mathematics of computerized tomography. Vol. 32 of Classics in applied mathematics. Society for Industrial and Applied Mathematics, Philadelphia.

[4] Radon, J., 1917. Über die Bestimmung von Funktionen durch ihre Integralwerte längs gewisser Mannigfaltigkeiten. Ber. Verh. Sächs. Akad. Wiss. Leipzig, Math. Nat. kl. 69, 262–277.
